# Supplementary material for: Growth modes of partially fluorinated organic molecules on amorphous silicon dioxide
Source: arXiv:2110.08289 source file (2021-10-15)
Supplement: Supplementary file 1 [file si.pdf]

# Supporting Information (SI) to Growth modes of partially fluorinated organic molecules on amorphous silicon dioxide

Mila Miletic,† Karol Palczynski,† and Joachim Dzubiella*,¶

†*Research Group Simulations of Energy Materials, Helmholtz-Zentrum Berlin fr Materialien und Energie, Hahn-Meitner-Platz 1, D-14109 Berlin, Germany*

‡*Institut für Physik, Humboldt-Universität zu Berlin, Newtonstr. 15, 12489 Berlin, Germany*

¶*Applied Theoretical Physics - Computational Physics, Albert-Ludwigs-Universität Freiburg, Hermann-Herder Straße 3, D-79104 Freiburg, Germany*

E-mail: joachim.dzubiella@physik.uni-freiburg.de

# Stochastic Integrator

For a smoother sampling of phase space it is of advantage to use a stochastic integrator for the simulation of the organic molecules. Here a friction and a noise term are added to the ordinary (Newton's) equations of motion resulting in the stochastic dynamics (SD) equation for the atomic positions $\vec{r}_i$

$$m_i \frac{\mathrm{d}^2 \vec{r}_i}{\mathrm{d}t^2} = -m_i \xi_i \frac{\mathrm{d}\vec{r}_i}{\mathrm{d}t} + \vec{F}_i + \vec{R}_i, \tag{1}$$

where $m_i$ is the atomic mass, $\xi_i$ is the friction constant, $F_i$ the force acting on atom $i$, and $\vec{R}_i\,(t)$ is a temperature- and friction-dependent white noise process giving the particles random accelerations. The value of $\xi_i = 1$ ps$^{-1}$ was empirically chosen to warrant an efficient equilibration of the studied systems.

# Force field parameters

The P, 2P-, 3P-, 4P- and 6P-molecules are atomistically resolved in our simulations, in which each carbon (C) or hydrogen (H) atom $i$ is represented by a point-mass $m_i$ and a partial charge $q_i$ attached to its center. The interactions between all atoms are described by a classical Hamiltonian employing Lennard-Jones (LJ) and Coulomb potentials for nonbonded interactions and harmonic potentials for the intramolecular bond-, angular- and dihedral interactions, respectively. We employ the General Amber Force Field (GAFF),[1] specially designed to be suitable for a wide variety of organic and aromatic compounds, with the Hamiltonian

$$\begin{aligned} H\left(\vec{r}_{ij}\right) &= 4\varepsilon_{ij}\left[\left(\frac{\sigma_{ij}}{r_{ij}}\right)^{12} - \left(\frac{\sigma_{ij}}{r_{ij}}\right)^{6}\right] + \frac{q_i q_j}{\varepsilon r_{ij}} \\ &\quad + \frac{1}{2}K_{ij}^{b}\left(r_{ij} - r_{\mathrm{eq}}\right)^2 + \frac{1}{2}K_{ijk}^{\theta}\left(\theta_{ijk} - \theta_{\mathrm{eq}}\right)^2 \\ &\quad + \frac{1}{2}K_{ijkl}^{\phi}\left[1 + \cos\left(n\phi_{ijkl} - \gamma\right)\right], \end{aligned} \tag{2}$$

where $\sigma_{ij}$ and $\varepsilon_{ij}$ are the LJ parameters derived by applying the Lorentz-Berthelot combination rules to the single particle LJ parameters and $q_i$ and $q_j$ are the partial charges of atoms $i$ and $j$. $K_{ij}^{b}$ and $K_{ijk}^{\theta}$ are force constants for the bond- and angle-interactions, and $r_{\text{eq}}$ and $\theta_{\text{eq}}$ are the equilibrium bond lengths and bond angles respectively. $K_{ijkl}^{\phi}$ is a dihedral parameter and $\phi_{ijkl}$ the corresponding dihedral angle, while $\gamma$ serves as a phase angle being either 0° or 180°. The multiplicity $n$ determines the number of local energy minima of the dihedral potential. Bonds are constrained by the LINCS[2] algorithm.

Also for the intermolecular Lennard-Jones interactions between the aromatic carbon atoms the force field parameters from GAFF are used. The partial charges are calculated using Gaussian 09[3] by employing the B3LYP functional with the cc-PVTZ basis set using the electrostatic potential fitting method (ESP).[4] They are explicitly listed in Tab. 3.

**Table 1: p-6P partial charge map obtained with electrostatic potential fitting (ESP)[4] at B3LYP/cc-PVTZ level of theory.**

| atom name | $q$[e] | atom name | $q$[e] | atom name | $q$[e] | atom name | $q$[e] |
|---|---|---|---|---|---|---|---|
| C1 | -0.12 | C17 | -0.16 | C33 | -0.13 | H49 | 0.12 |
| C2 | -0.13 | C18 | -0.16 | C34 | -0.12 | H50 | 0.12 |
| C3 | -0.15 | C19 | 0.08 | C35 | -0.13 | H51 | 0.12 |
| C4 | 0.11 | C20 | -0.16 | C36 | -0.15 | H52 | 0.12 |
| C5 | -0.15 | C21 | -0.16 | H37 | 0.12 | H53 | 0.12 |
| C6 | -0.13 | C22 | 0.08 | H38 | 0.11 | H54 | 0.12 |
| C7 | 0.04 | C23 | -0.16 | H39 | 0.12 | H55 | 0.11 |
| C8 | -0.13 | C24 | -0.16 | H40 | 0.12 | H56 | 0.12 |
| C9 | -0.17 | C25 | 0.09 | H41 | 0.11 | H57 | 0.11 |
| C10 | 0.09 | C26 | -0.17 | H42 | 0.11 | H58 | 0.11 |
| C11 | -0.17 | C27 | -0.13 | H43 | 0.12 | H59 | 0.12 |
| C12 | -0.13 | C28 | 0.04 | H44 | 0.11 | H60 | 0.12 |
| C13 | 0.08 | C29 | -0.13 | H45 | 0.12 | H61 | 0.12 |
| C14 | -0.16 | C30 | -0.17 | H46 | 0.12 | H62 | 0.11 |
| C15 | -0.16 | C31 | 0.11 | H47 | 0.12 | | |
| C16 | 0.08 | C32 | -0.15 | H48 | 0.12 | | |

**Table 2: p-6P4F partial charge map obtained with electrostatic potential fitting (ESP)[4] at B3LYP/cc-PVTZ level of theory.**

| atom name | $q$[e] | atom name | $q$[e] | atom name | $q$[e] | atom name | $q$[e] |
|---|---|---|---|---|---|---|---|
| C1 | -0.47 | C17 | -0.16 | C33 | 0.44 | H49 | 0.12 |
| C2 | 0.44 | C18 | -0.16 | C34 | -0.47 | H50 | 0.12 |
| C3 | -0.39 | C19 | 0.08 | C35 | 0.44 | H51 | 0.12 |
| C4 | 0.12 | C20 | -0.16 | C36 | -0.39 | H52 | 0.12 |
| C5 | -0.39 | C21 | -0.16 | F37 | -0.20 | H53 | 0.12 |
| C6 | 0.44 | C22 | 0.09 | H38 | 0.18 | H54 | 0.12 |
| C7 | 0.20 | C23 | -0.16 | H39 | 0.22 | H55 | 0.14 |
| C8 | -0.23 | C24 | -0.16 | F40 | -0.20 | H56 | 0.12 |
| C9 | -0.13 | C25 | 0.06 | H41 | 0.18 | H57 | 0.14 |
| C10 | 0.05 | C26 | -0.13 | H42 | 0.14 | H58 | 0.18 |
| C11 | -0.13 | C27 | -0.22 | H43 | 0.12 | F59 | -0.20 |
| C12 | -0.23 | C28 | 0.19 | H44 | 0.14 | H60 | 0.22 |
| C13 | 0.09 | C29 | -0.22 | H45 | 0.12 | F61 | -0.20 |
| C14 | -0.16 | C30 | -0.13 | H46 | 0.12 | H62 | 0.18 |
| C15 | -0.16 | C31 | 0.12 | H47 | 0.12 | | |
| C16 | 0.08 | C32 | -0.39 | H48 | 0.12 | | |

**Table 3: Partial charges of the surface atoms taken from Ref.[5]**

| atom name | $q$[e] |
|---|---|
| Si | 2.10 |
| O | -1.05 |

## Influence of the interaction cutoff on the growth dynamics

We examine the influence of specific simulation input parameters on the growth dynamics of the molecules. First, we examine the influence of the short-range interaction cutoff. Figure 1 is showing simulation snapshots for three different cutoff values. In all three cases, we observe the formation of a wetting layer (layer of lying molecules) at the interface. However, the critical coverage that is necessary for the molecules to achieve the orientational change from the lying to the upright standing configuration, differs between the interaction cutoffs: while in the case of $r_{\mathrm{cut}} = 1.5$ nm we observe the collective reorientation of molecules after the critical coverage is achieved, in the case of $r_{\mathrm{cut}} = 0.9$ and 1.2 nm we observe the formation of bimodal phases - the simultaneous existence of stable upright standing molecular clusters together with clusters consisting of lying molecules. For the highest used cutoff distance of $r_{\mathrm{cut}} = 1.5$ nm the average inclination angle is higher compared to the cases with lower cutoffs used, after the first monolayer is completed (Figure 2 a)). These results exemplify the sensitivty of growth dynamics on the interaction cutoffs.

If we now study the increase in average hight of the formed layer with the number of deposited molecules (see Figure 2 b)), we see that the average height reaches 2.3 nm after the first layer is finished, close to the end-to-end length of the individual molecule, 2.45 nm, but still lower as the molecules are not fully perpendicular with their LMA to the surface plane. The average height in case of $r_{\mathrm{cut}} = 0.9$ nm is higher due to more molecules participating in the wetting layer. Conclusively, for the growth simulations we opt for the cutoff distance of $r_{\mathrm{cut}} = 1.3$ nm, as it yields similar results as the larger cutoff of $r_{\mathrm{cut}} = 1.5$ nm. This is a good compromise between accuracy and the computational cost.

## Influence of the deposition rate on growth dynamics

In this chapter we discuss the influence of the attempted deposition rates on the growth dynamics of the molecules. The deposition process was simulated with three different deposition rates: $3000^{-1}$ ps$^{-1}$, $300^{-1}$ ps$^{-1}$ and $30^{-1}$ ps$^{-1}$. Results obtained by depositing

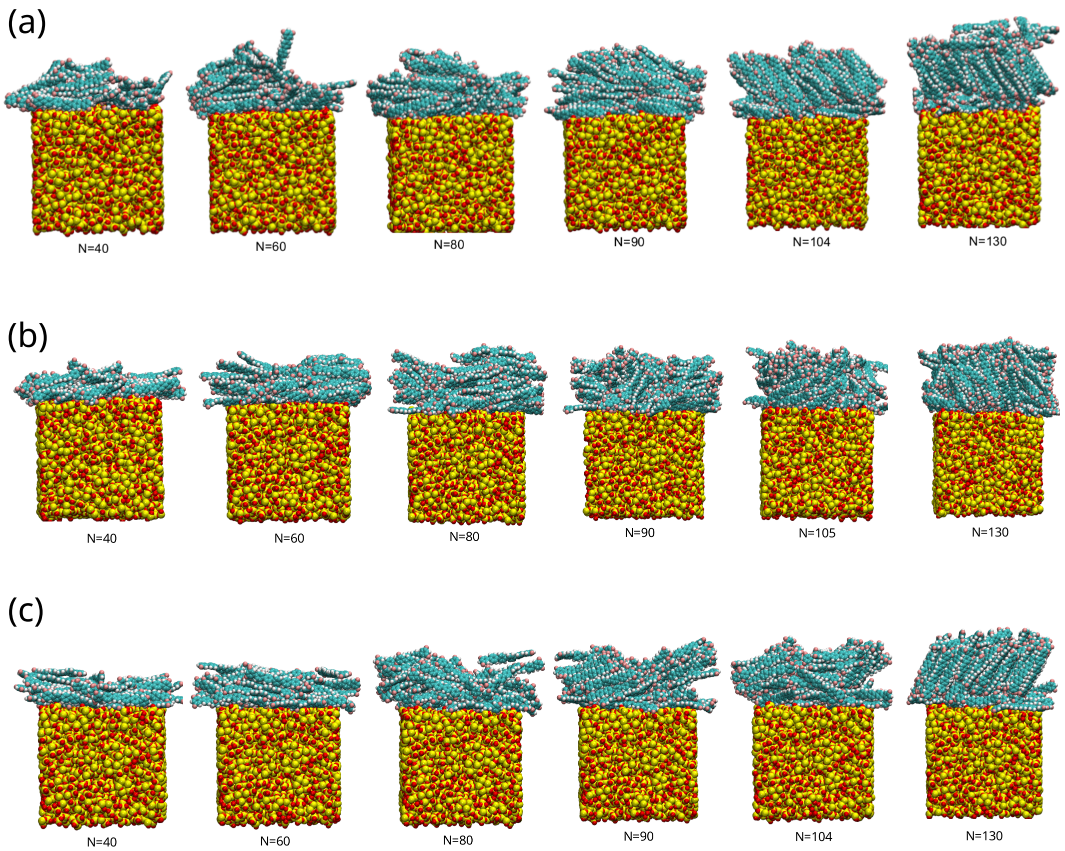


Figure 1: Snapshots of $p$-6P4F growth at $T = 575$ K for cutoff distances of a) $r_{\text{cut}} = 0.9$ nm, b) $r_{\text{cut}} = 1.2$ nm and c) $r_{\text{cut}} = 1.5$ nm.

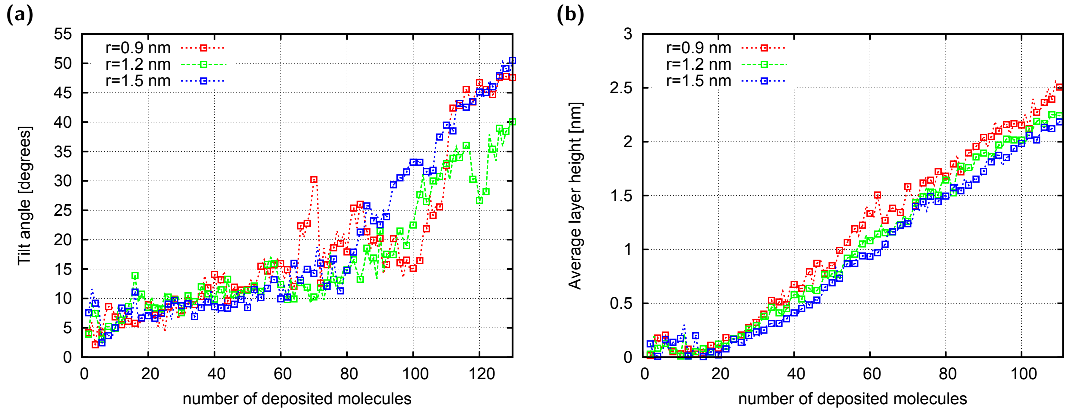


Figure 2: The dependence of the a) average inclination angle and b) average layer height on the number of deposited molecules and chosen cutoff distance at $T = 575$ K.

molecules every 30 ps do not result in uniform, layer-by-layer growth, as observed for lower deposition rates (see Figure 4).

The underlying reason for this is that the timescale of 30 ps is between 1 and 2 orders

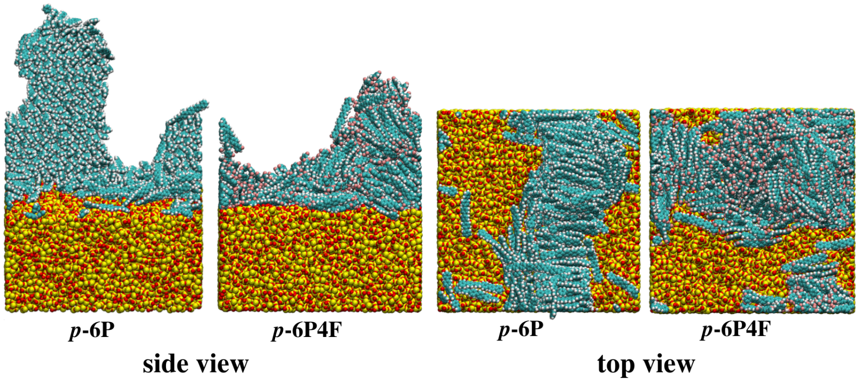


Figure 3: Snapshots of the $p$-6P and $p$-6P4F growth at $T = 575$ K for the deposition rate of 30 ps.

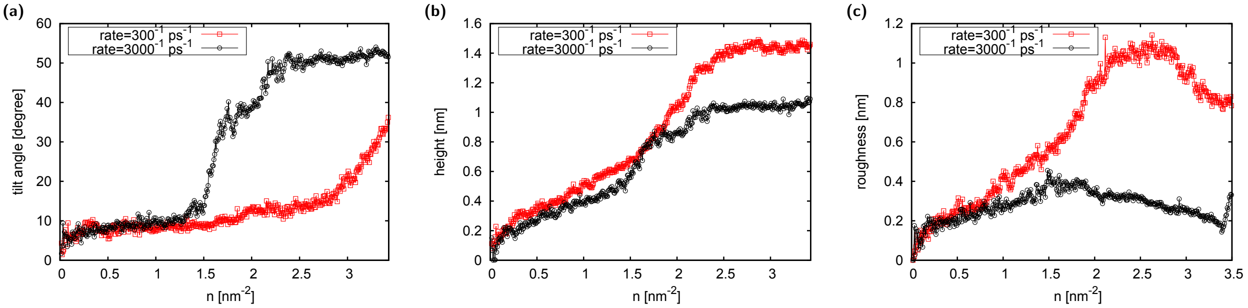


Figure 4: Average a) inclination angle, b) height and c) monolayer roughness as a function of surface number density for the $p$-6P, compared between the two deposition rates of $3000^{-1}$ ps$^{-1}$ and $300^{-1}$ ps$^{-1}$ at $T = 575$ K.

of magnitude lower than the observed diffusion time scale. This prevents the molecule once it is deposited from diffusing to one of the existing islands or ascending over the terrace to integrate into the existing layer, before the next molecule is deposited. This results in the formation of amorphous clusters on the surface, even with a surface density of $n$=3.04 nm$^{-2}$ for both $p$-6P and $p$-6P4F. Fig. 4 compares the results for the average inclination angle, monolayer height and roughness between the deposition rates of $3000^{-1}$ ps$^{-1}$ and $300^{-1}$ ps$^{-1}$ at $T = 575$ K, in case of the $p$-6P and $p$-6P4F.

Furthermore, as the deposition rate decreases from $300^{-1}$ ps$^{-1}$ to $3000^{-1}$ ps$^{-1}$, the critical surface density necessary for the molecules to have an orientational change from a lying to an upright standing configuration decreases: Decreasing the rate by one order of magnitude results in the critical surface density decrease from about 350 to about 200 molecules (in

this case we define the critical cluster as the cluster comprising upright standing molecules). Lower deposition rates enable proper system equilibration and allow molecules to diffuse to nearby cluster units and bind to them. Once the clusters become big enough, the number of upright standing molecules increases until it becomes energetically favorable for the other molecules to stand up as well.

In case of the deposition rate of $3000^{-1}$ $ps^{-1}$, after the surface density of $n$=1.52 $nm^{-2}$ and $n$=1.75 $nm^{-2}$ for the $p$-6P and $p$-6P4F, respectively, is reached, they start forming stable, upright standing molecular clusters. In case of the deposition rate of $300^{-1}$ $ps^{-1}$, larger surface densities are required to observe the orientational change ($n$=3.04 $nm^{-2}$ for the $p$-6P and $n$=2.66 $nm^{-2}$ for the $p$-6P4F). In case of the $p$-6P the existence of bimodal phases (phases containing both lying and upright standing molecules) is observed after $n$=3.80 $nm^{-2}$. As the deposition continues and reaches $n$=4.18 $nm^{-2}$ for the $p$-6P and $n$=3.88 $nm^{-2}$ for the $p$-6P4F, all molecules (besides the wetting layer which is about 6% and 4% of the first monolayer (1ML) in case of $p$-6P and $p$-6P4F, respectively) have the upright standing orientation, with an average inclination angle of about 54° and 68°.

## Surface diffusion analysis

As molecules are deposited one by one on the surface, each molecule diffuses on the surface before it eventually integrates into the nearest molecular cluster. Thus, understanding the subtle differences in diffusion between the $p$-6P and $p$-6P4F can help us to understand the differences in the growth modes between $p$-6P and $p$-6P4F. The total long-time diffusion coefficients, $D^{\mathrm{tot}}$, averaged over the $x$- and $y$-direction of the molecular motion, are obtained from the mean squared displacements (MSDs) of the molecular COM from the simulated trajectories, via

$$\left\langle [x(t)-x(t_0)]^2+[y(t)-y(t_0)]^2 \right\rangle = \lim_{t\to\infty} 4D^{\mathrm{tot}}t. \tag{3}$$

where $x(t)$ and $y(t)$ is the coordinates of the molecular COM at time $t$ and $\langle\rangle$ denotes the ensemble average. We observed that the diffusion coefficients follow the Arrhenius law with temperature:

$$D^{\text{tot}}(T) = D_0 \exp\left(-\frac{\Delta E}{k_B T}\right). \tag{4}$$

where $D_0$ is the pre-exponential factor, $k_B$ is Boltzmann constant, and $T$ is temperature. The diffusion energy barrier $\Delta E$ in the exponent can be extracted from the knowledge of the diffusion at different temperatures, shown in Figure 5. Diffusion coefficients on the respective first monolayers are almost one order of magnitude higher than on the silica surface. Furthermore, the surface diffusion coefficients of the $p$-6P4F are lower compared to diffusion coefficients of $p$-6P on both surfaces, which correlates with the higher binding free energies of $p$-6P4F to the underlying substrates. We estimated $\Delta E$ for the $p$-6P in our previous work[6] to be 67.41 kJ/mol, while $\Delta E$ for the $p$-6P4F amounts to 81.62 kJ/mol on silica. On the first monolayers, the diffusion energy barriers are significantly lower and amount to 19.80 kJ/mol for the $p$-6P4F and 14.02 kJ/mol for the $p$-6P, which is roughly 50% of their respective surface binding energies.

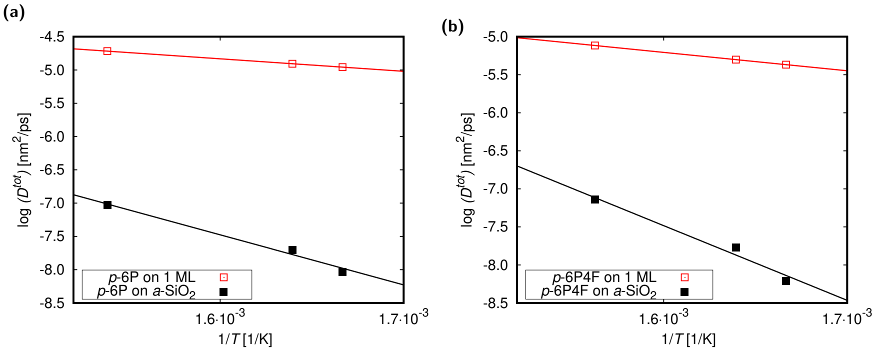


Figure 5: Logarithm of the diffusion coefficients as a function of the inverse temperature for the a) $p$-6P and b) $p$-6P4F on silica and its respective first monolayers. From the linear fits of the Arrhenius equation to the temperature-dependent diffusion coefficients, the effective energy barrier can be estimated.

# References


(1) Wang, J.; Wolf, R. M.; Caldwell, J. W.; Kollman, P. A.; Case, D. A. Development and Testing of a General Amber Force Field. *J. Comput. Chem.* **2004**, *25*, 1157–1174.

(2) Hess, B.; Bekker, H.; Berendsen, H. J. C.; Fraaije, J. G. E. M. LINCS: a Linear Constraint Solver for Molecular Simulations. *J. Comput. Chem.* **1997**, *18*, 1463–1472.

(3) Frisch, M. J.; Trucks, G. W.; Schlegel, H. B.; Scuseria, G. E.; Robb, M. A.; Cheeseman, J. R.; Scalmani, G.; Barone, V.; Mennucci, B.; Petersson, G. A. et al. Gaussian 09 Revision D.01. Gaussian Inc. Wallingford CT 2009.

(4) Besler, B. H.; Merz, K. M.; Kollman, P. A. Atomic Charges Derived from Semi-empirical Methods. *J. Comput. Chem.* **1990**, *11*, 341.

(5) Skelton, A. A.; Fenter, P.; Kubicki, J. D.; Wesolowski, D. J.; Cummings, P. T. Simulations of the Quartz(1011)/Water Interface: A Comparison of Classical Force Fields, Ab Initio Molecular Dynamics, and X-ray Reflectivity Experiments. *The Journal of Physical Chemistry C* **2011**, *115*, 2076–2088.

(6) Miletic, M.; Palczynski, K.; Dzubiella, J. Quantifying entropic barriers in single-molecule surface diffusion. *The Journal of Chemical Physics* **2020**, *153*, 164713.
